# Supplementary material for: qs$GW$ quasiparticle and $GW$-BSE excitation energies of 133,885 molecules
Source: arXiv:2512.10815 ancillary file (2025-12-11)
Supplement: Supplementary file 1 [file SI.pdf]

Supporting Information

# qs$GW$ quasiparticle and $GW$-BSE excitation energies of 133 885 molecules

Dario Baum, Arno Förster, Lucas Visscher

## Example ADF Input File Initial Calculations

```
Task SinglePoint

system
  Atoms
            H       1.0151783459      -0.0657170576       0.0000000000
            O       0.0505387116       0.0505387116       0.0000000000
            H      -0.0657170576       1.0151783459       0.0000000000
  End
End

Engine adf
  basis
    core None
    type Corr/TZ3P
  End
  dependency
    bas 0.005
  End
  excitations
    bse True
    iterations 20
    lowest 5
  End
  gw
    nstates -1
    selfconsistency qsGW
  End
  numericalquality Good
  relativity
    level None
  End
  rihartreefock
    dependencythreshold 0.005
  End
  symmetry nosym
  xc
    libxc BHandHLYP
  End
EndEngine
```

## Example ADF Input File Restart Calculations

```
Task SinglePoint

system
  Atoms
            H       1.0151783459      -0.0657170576       0.0000000000
            O       0.0505387116       0.0505387116       0.0000000000
            H      -0.0657170576       1.0151783459       0.0000000000
  End
End

Engine adf
  basis
    core None
    type Corr/TZ3P
  End
  dependency
    bas 0.001
  End
  excitations
    bse True
    iterations 20
    lowest 5
  End
  gw
    nstates -1
    selfconsistency qsGW
  End
  numericalquality VeryGood
  relativity
    level None
  End
  rihartreefock
    dependencythreshold 0.001
  End
  symmetry nosym
  xc
    libxc BHandHLYP
  End
EndEngine
```
